# Supplementary material for: Invariant expansion of the 30-band k.p model and its parameters for III-V compounds
Source: arXiv:2201.03234 source file (2022-01-10)
Supplement: Supplementary file 1 [file Supplementary.pdf]

# Supplementary Material for: Invariant expansion of the 30-band $\boldsymbol{k}\cdot\boldsymbol{p}$ model and its parameters for III-V compounds

Krzysztof Gawarecki,[1,*] Paweł Scharoch,[2] Michał Wiśniewski,[3] Jakub Ziembicki,[2] Herbert S. Mączko,[2] Marta Gładysiewicz,[3] and Robert Kudrawiec[2]

[1]*Department of Theoretical Physics, Wrocław University of Science and Technology, Wybrzeże Wyspiańskiego 27, 50-370 Wrocław, Poland*

[2]*Department of Semiconductor Materials Engineering, Wrocław University of Science and Technology, Wybrzeże Wyspiańskiego 27, 50-370 Wrocław, Poland*

[3]*Department of Experimental Physics, Wrocław University of Science and Technology, Wybrzeże Wyspiańskiego 27, 50-370 Wrocław, Poland*

This Supplementary Material contains figures for band structures of all the materials considered in the main part of the manuscript.

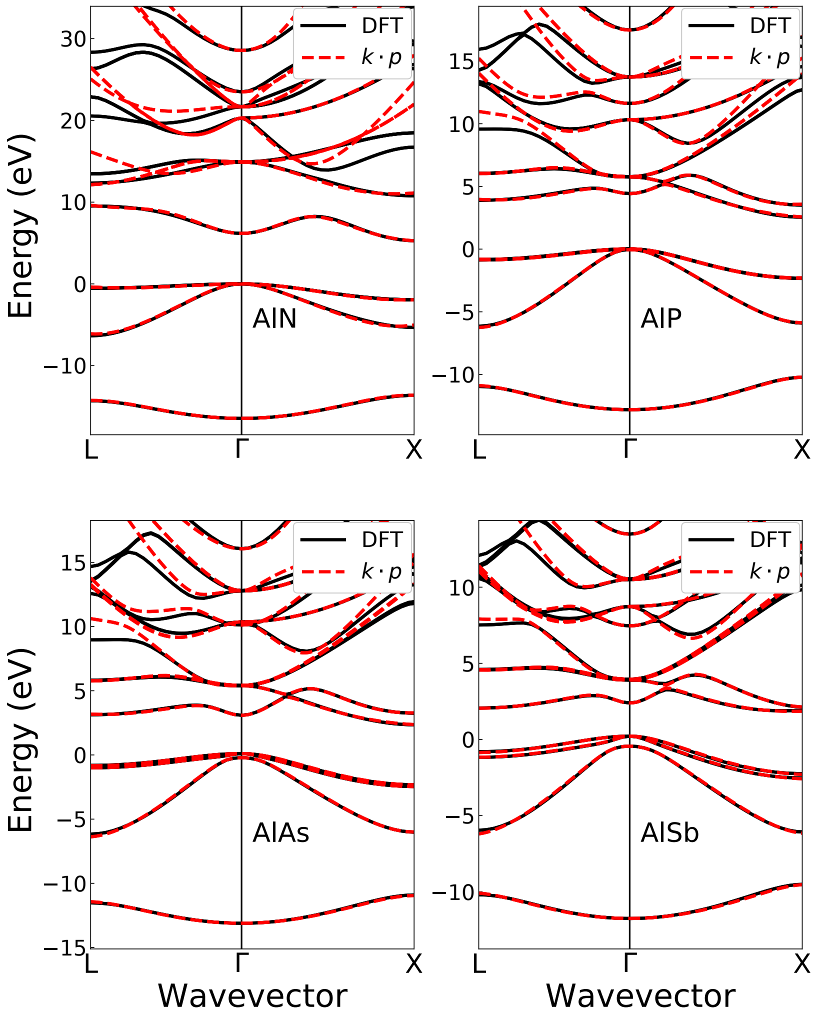


* Krzysztof.Gawarecki@pwr.edu.pl

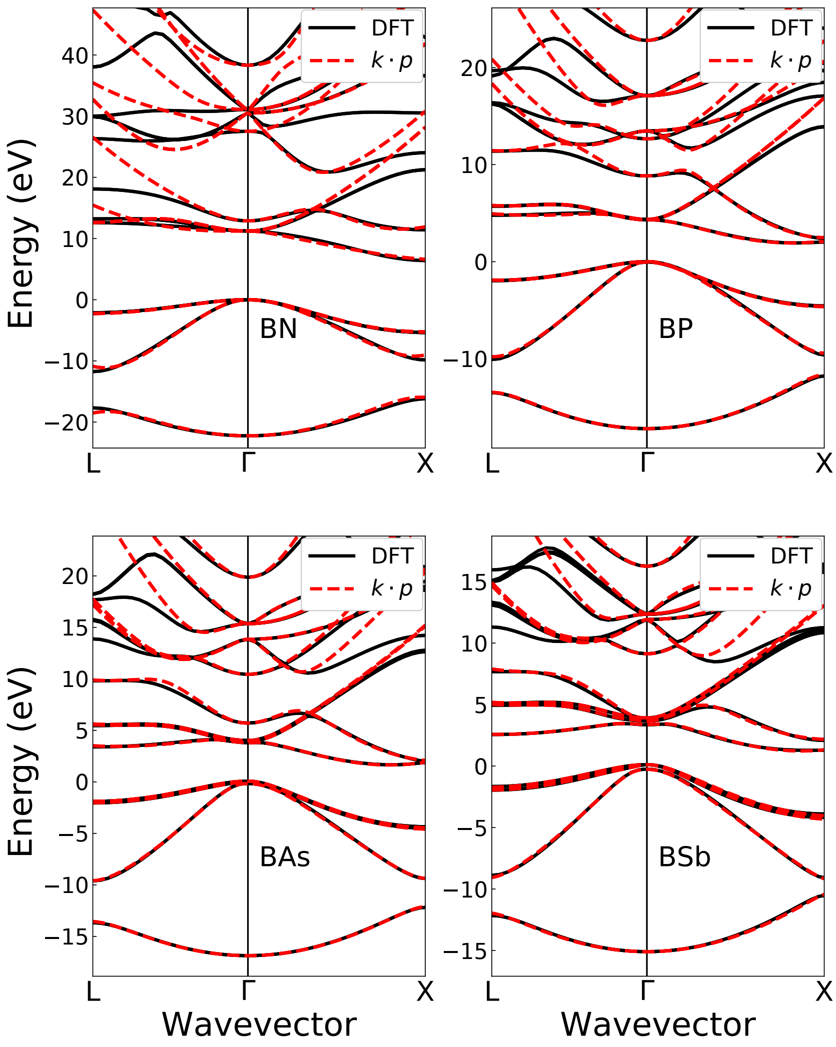
DFT
$k \cdot p$
BN
BP
BAs
BSb
Energy (eV)
Wavevector
L
Γ
X

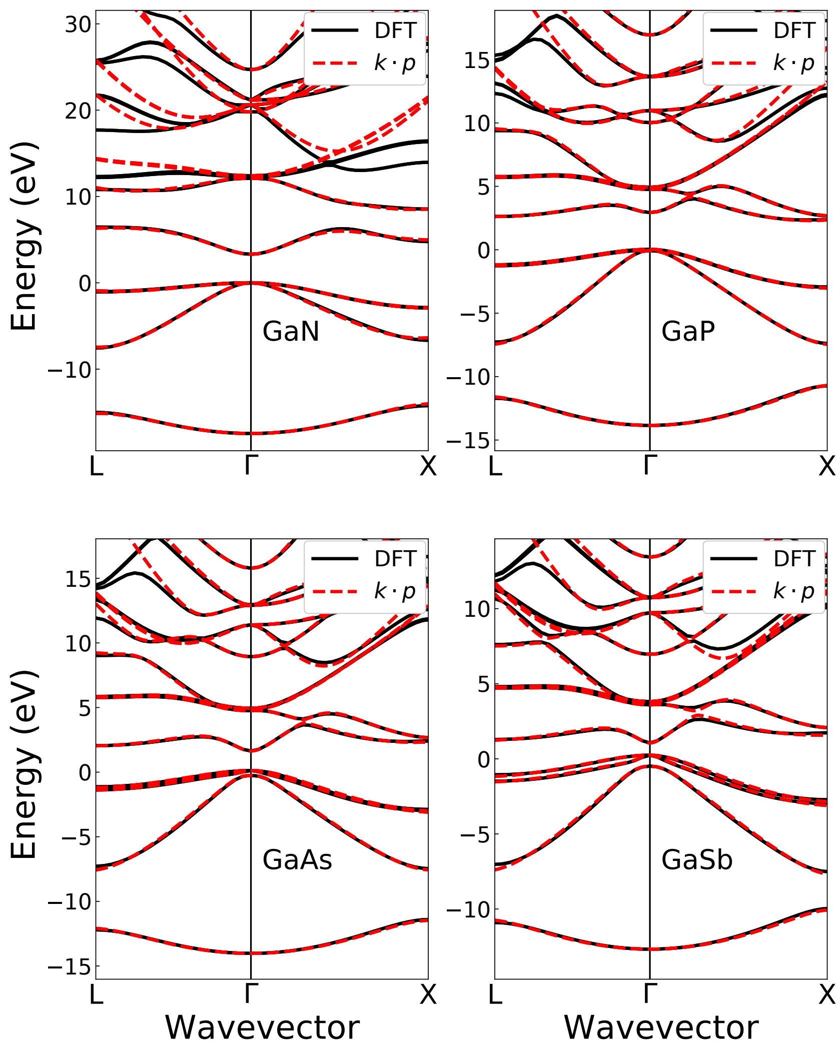

DFT
$k \cdot p$
GaN
GaP
GaAs
GaSb
Energy (eV)
Wavevector
L
Γ
X
30
20
10
0
−10
15
5
−5
−15

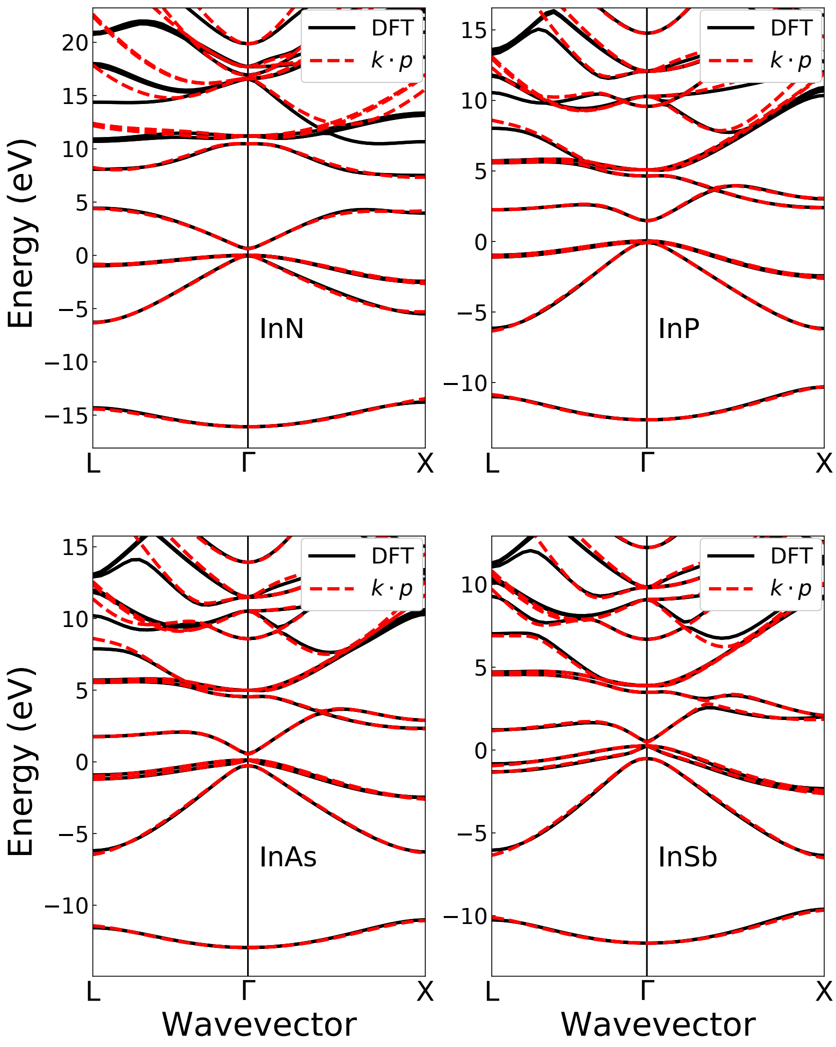

DFT
$k \cdot p$
InN
InP
InAs
InSb
Energy (eV)
Wavevector
L
Γ
X
